# Supplementary material for: Measuring Your ASTE Models in The Wild: A Diversified Multi-domain Dataset For Aspect Sentiment Triplet Extraction
Source: arXiv:2305.17448 source file (2023-05-27)
Supplement: Supplementary file 1 [file dataset.tex]

% \section{Dataset}
% \subsection{Comparison}\XT{->footnote in the appendix}
% Since aspect quadruples \textit{(aspect term, aspect category, opinion term, sentiment polarity)} can be transformed into aspect triplets. In this section, we remove the aspect category and transform existing quadruple datasets \citep{cai-etal-2021-aspect, zhang-etal-2021-aspect-sentiment} into triplets datasets. Then we compare \dataset with these datasets in Table \ref{tab:app-cmp}. The results show that \dataset has more domains, more diversified sentence lengths, more complex sentence patterns, and more implicit aspects than existing aspect quadruple datasets. Thus, the advantages of \dataset still hold when compared with quadruple datasets. It is worth noting that \citet{cai-etal-2021-aspect} annotate both implicit aspects and opinions in the quadruple. We exclude implicit opinions because \textit{"(NULL, NULL, POS/NEG/NEU)"} contains little sentimental information.

\section{Dataset}
\label{sec:app-dataset}
\subsection{Dataset Details}
\paragraph{Domain Selection Process.} First, we select the most popular four domains based on the best seller report of Amazon and Internet. For these four domains, we annotate more data to enable research on ASTE with more realistic and representative reviews. Then, to enable more comprehensive research like the cross-domain setting, we randomly select another four domains and annotate less data for test in the cross-domain setting. 
\paragraph{Annotator compensation.} As described in Section \ref{sec:annotation}, we hire 18 workers in the annotation and follow strict quality control to ensure the quality of the annotation. We ensure the privacy right of workers are respected in the annotation process.
All workers have been paid above the local minimum wage and agreed to use the dataset for research purposes.
\paragraph{License.}\dataset will be publicly avaliable under the terms of \href{https://www.wikidata.org/wiki/Q42553662}{CC BY-NC-SA 4.0 License}. The dataset is for academic use, which is consistent with its origination dataset Amazon \citep{ni2019justifying}.

We sample two instances for each domain and demonstrate them in Table \ref{tab:app-case}. The first column displays the review text. And the second column shows the extracted triplets (aspect terms, opinion terms, sentiment polarity).
