# Supplementary material for: Measuring Your ASTE Models in The Wild: A Diversified Multi-domain Dataset For Aspect Sentiment Triplet Extraction
Source: arXiv:2305.17448 source file (2023-05-27)
Supplement: Supplementary file 2 [file in-domain.tex]

\subsection{In-domain Experiments}
\label{sec:app-in-domain}

Table \ref{tab:in-domain} shows the overall comparison results on in-domain ASTE where the training data and test data are from the same domain. We can observe that: (1) Span-ASTE performs the best on \dataset and achieves comparable results with GAS on \citet{xu-etal-2020-position}. (2) The performance of the four models on the dataset of \citet{xu-etal-2020-position} is better than on \datasetwb, which indicates that \dataset introduces more challenges to the ASTE research empirically. (3) Among the four domains in \datasetwb, models perform consistently the best in the fashion domain and the worst in the beauty domain.

% \subsection{Challenges from ASTE}
\begin{figure*}
     \centering
     \begin{subfigure}[b]{0.32\textwidth}
         \centering
         \includegraphics[width=\textwidth]{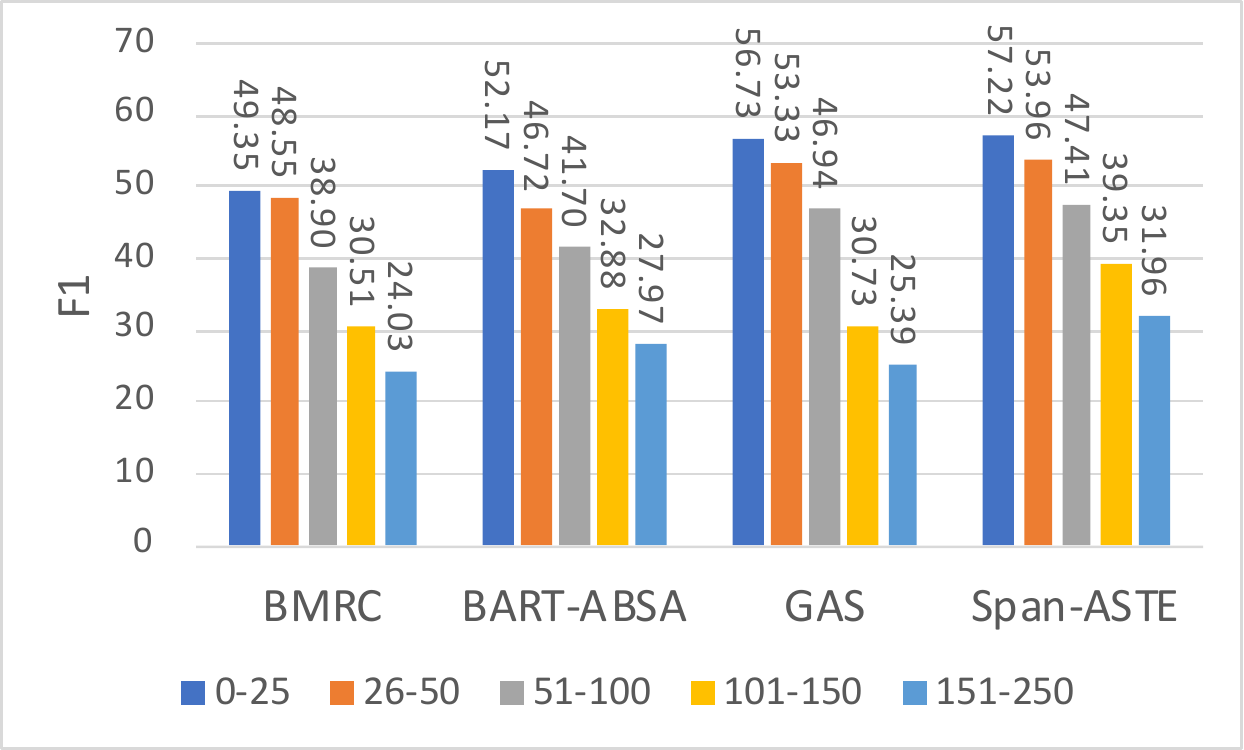}
         \caption{F1 scores on reviews of different lengths.}
         \label{fig:analyse-indomain-length}
     \end{subfigure}
        \hfill
     \begin{subfigure}[b]{0.32\textwidth}
         \centering
         \includegraphics[width=\textwidth]{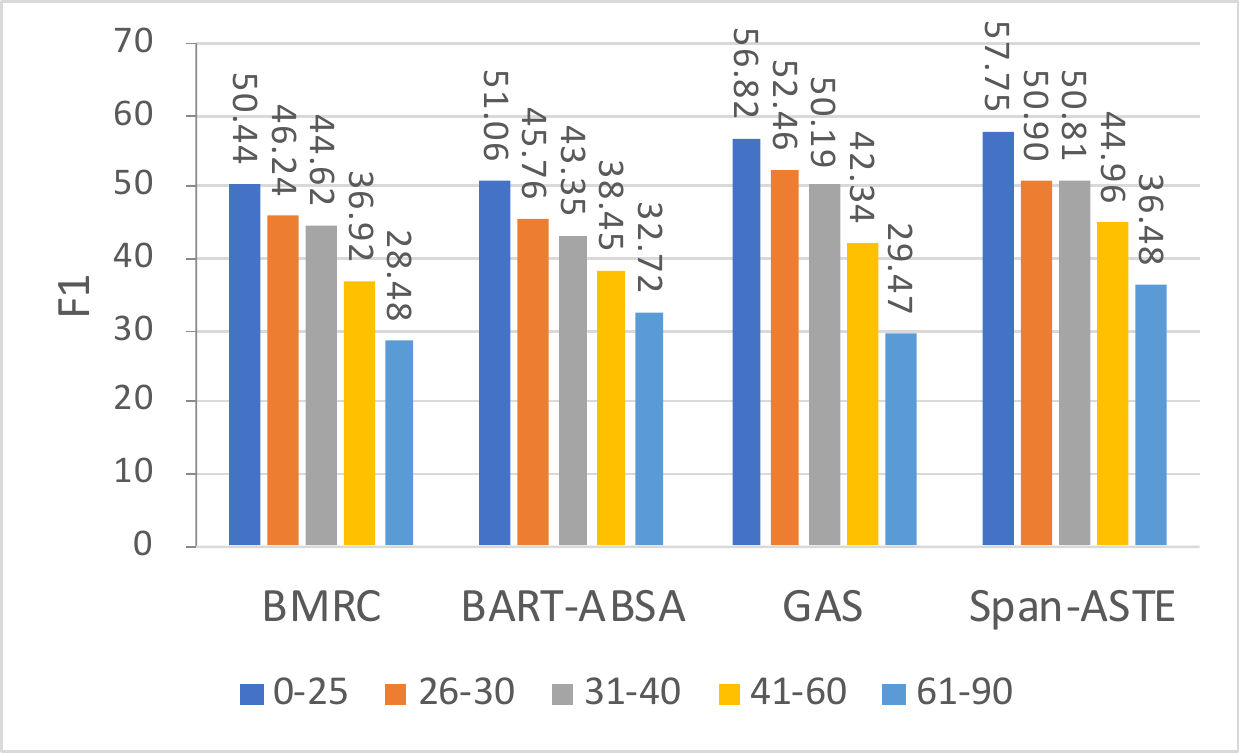}
         \caption{F1 scores on reviews of different numbers of POS 2-grams.}
         \label{fig:analyse-indomain-pos}
     \end{subfigure}
     \hfill
     \begin{subfigure}[b]{0.32\textwidth}
         \centering
         \includegraphics[width=\textwidth]{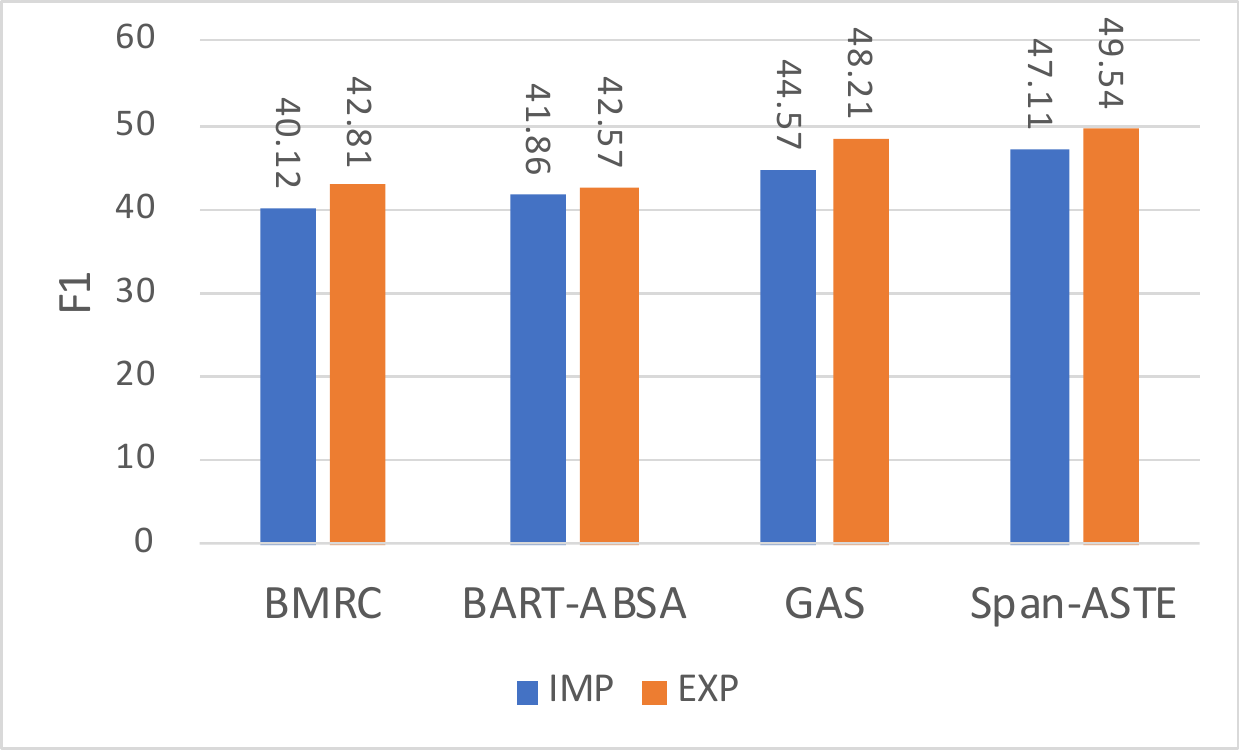}
         \caption{F1 scores on reviews of different aspect types.}
         \label{fig:analyse-indomain-imp}
     \end{subfigure}
        \caption{F1 scores on different review lengths, different numbers of POS 2-grams, and different aspect types. The results are average F1 scores on the four source domains. We can conclude that long reviews, complex sentences, and implicit aspect terms make \dataset more challenging. }
        \label{fig:analyse-indomain-ins}
\end{figure*}

Compared with ASTE results in previous works \citep{xu-etal-2021-learning}, we can observe the performance drop in Table \ref{tab:in-domain}. So we further analyze the challenges in \dataset by comparing the performance under different review lengths, sentence complexity, and aspect types as shown in Figure \ref{fig:analyse-ins}.  All the results are average F1 scores of 16 transfer pairs in the single-source cross-domain setting.
\begin{itemize}
    \item \textbf{Length.} As shown in Figure \ref{fig:analyse-indomain-ins}(a), we categorize the instance by its length and test the model for each category. We can observe that the longer the instance, the worse the model performance. Since \dataset contains reviews of various lengths, this characteristic introduces more challenges to the task.
    \item \textbf{Sentence Complexity.} We represent sentence complexity by the number of 2-grams in the POS sequence of the review text. Then we explore the relationship between extraction performance and sentence complexity. Figure \ref{fig:analyse-indomain-ins}(b) shows that the performance decreases with the sentence complexity increases.
    % In Figure (\ref{fig:analyse-pos}), we investigate the performance of the model when the number of triplets ranges from 1 to 7. We find that the performance of the model first increases and then decreases with the number of triplets growing. \XT{TBD}
    % \XT{reasons}
    \item \textbf{Aspect Types.} In Figure \ref{fig:analyse-indomain-ins}(c), we compare the F1 results of triplets with implicit and explicit aspect terms. The results suggest that the implicit aspect term is harder for the model than the explicit one. 
    \dataset includes both implicit and explicit aspects terms. It makes \dataset more challenging.
    % Because the implicit aspect can refer to any attribute of the product which introduces ambiguity in the extraction process. 
\end{itemize}
We can conclude that long reviews, complex sentences, and implicit aspect terms make \dataset a challenging dataset.
